# Supplementary material for: FunMap: Efficient Execution of Functional Mappings for Knowledge Graph Creation
Source: arXiv:2008.13482 source file (2020-10-05)
Supplement: Supplementary file 1 [file 6appendix.tex]

\section{Appendix}
\label{sec:appendix}
\begin{lstlisting}[]
File := <SetTriplesMap>  
SetTriplesMap := <TriplesMap>*
TriplesMap :=   a rr:TriplesMap
                <TriplesMapID>
                rml:logicalSource <logicalMap>
                (rr:subjectMap ( <subjectMap> | <FunctionMap> ) |
                rr:subject (IRI|Literal) )
                ( rr:predicateObjectMap <predicateObjectMap> )*
logicalMap :=   a rml:logicalSource
                rml:source
                ( rml:referenceFormulation ql:(CSV|XPath|JSONPath) )?
                ( rml:iterator RefType )?
subjectMap :=   a rr:TermMap
                a rr:subjectMap
                ( rr:template StringTemplate  | 
                rml:reference ValueRef  )
predicateObjectMap :=   a rr:predicateObjectMap
                    ( rr:predicateMap <predicateMap> | 
                    rr:predicate IRI )+
                    ( rr:objectMap ( <objectMap> | <FunctionMap> ) |
                    rr:object (IRI|Literal) )+
Execution :=    a fno:Execution
                fno:executes <Function>
Function :=     a fno:Function
                fno:name String
                fno:expects <Parameters>
                fno:returns <Output>
Parameters :=   ( fno:predicate IRI )+
                ( fno:required Literal )*
                (rr:objectMap <objectMap> )+ 
Output :=   ( fno:predicate IRI )+
            ( fno:required Literal )*
            ( rr:objectMap <objectMap> )+
objectMap :=    a rr:TermMap
                a rr:objectMap
                ( rr:template StringTemplate | 
                rml:reference ValueRef |
                rr:RefObjectMap <RefObjectMap> )
refObjectMap := a rr:RefObjectMap
                ( rr:parentTriplesMap <TriplesMap> )+
                ( rr:joinCondition <joinCondition> )*
joinCondition :=    a rr:joinCondition
                    rr:child ( ValueRef | <FunctionMap> )
                    rr:parent ( ValueRef | <FunctionMap> )
predicateMap := a rr:TermMap
                a rr:predicateMap
                ( rr:template StringTemplate | 
                rml:reference ValueRef )
FunctionMap :=  a rr:TermMap
                a fnml:FunctionTermMap 
                fnml:functionValue (rml:logicalSource <logicalMap> +
                rr:predicateObjectMap <Execution> +
                rr:predicateObjectMap <Parameters> )	                
\end{lstlisting}
\item \textbf{Action B related to production} \begin{lstlisting} 
    triplesMap :=   a rr:TriplesMap
                    rml:logicalSource <logicalMap>
                    rr:subjectMap <FunctionMap>
    \end{lstlisting}
    \textbf{is defined as:}
    \begin{lstlisting}
    {File.output = SetTriplesMap.TriplesmapValue + File.NewOutput
    File.NewOutput = NewSetTriplesMap.NewTriplesMapValue
    
    NewSetTriplesMap.NewTriplesMapValue = 
                        TriplesMap.NewTriplesMapValue + 
                        NewSetTriplesMap.NewTriplesMapValue

    TriplesMap.NewTriplesMapValue = 
                        NewTriplesMapID + logicalSource.NewSourceValue +
                        subjectMap.NewSubjectMapValue + 
                        objectMap.objectMapValue 

    logicalSource.NewSourceValue = source.NewValue + 
                            ( ql.Value | \epsilon ) + ( iterator.Value | \epsilon ) 

    subjectMap.NewSubjectMapValue = template.prefixValue + 
                                    Output.objectMapValue

    objectMap.objectMapValue = RefObjectMap.RefObjectMapValue

    RefObjectMap.RefObjectMapValue = parentTriplesMap.TriplesMapValue +
                                    joinCondition.joinConditionValue
                                    
    joinCondition.joinConditionValue = child.Value + parent.Value

    child.Value = Parameters.objectMapValue
    parent.Value = Parameters.objectMapValue}
    \end{lstlisting}
    \item \textbf{Action C related to production} \begin{lstlisting} 
	rr:predicateObjectMap <predicateObjectMap>
    predicateObjectMap :=	a rr:predicateObjectMap
    ( rr:predicateMap <predicateMap> | rr:predicate IRI )+
    ( rr:objectMap ( <objectMap> | <FunctionMap> ) |
    rr:object (IRI|Literal) )+
    \end{lstlisting}
    \textbf{is as:}
    \begin{lstlisting}
    {subjectMap.subjectMapValue = 
                    (objectMap.firstObjectMapValue | object.firstValue)}
    {NewSetTriplesMap.NewTriplesMapValue = 
                    NewSetTriplesMapID + logicalSource.SourceValue +
                    SetSubjectMap.NewSubjectMapValue + \epsilon
                
    SetSubjectMap.NewSubjectMapValue = 
                    (objectMap.SetObjectMapValue | object.SetValue)}
    \end{lstlisting}
